# Supplementary material for: Ab Initio Derivation of Model Energy Density Functionals
Source: arXiv:1507.00697 source file (2015-07-07)
Supplement: Supplementary file 1 [file abi-supp-11.pdf]

# Supplemental material for: Ab Initio Derivation of Model Energy Density Functionals

Jacek Dobaczewski<sup>1,2,3,4</sup>

<sup>1</sup>*Department of Physics, University of York, Heslington, York YO10 5DD, United Kingdom*

<sup>2</sup>*Department of Physics, P.O. Box 35 (YFL), University of Jyväskylä, FI-40014 Jyväskylä, Finland*

<sup>3</sup>*Institute of Theoretical Physics, Faculty of Physics,*

*University of Warsaw, Pasteura 5, PL-02-093 Warsaw, Poland*

<sup>4</sup>*Helsinki Institute of Physics, P.O. Box 64, FI-00014 Helsinki, Finland*

PACS numbers: 21.60.Jz, 21.60.De, 21.10.Dr

## NUMERICAL PARAMETERS

Numerical calculations presented in this study were performed by employing the code HFODD (v2.75c) [1] and using the spherical harmonic-oscillator (HO) basis of  $N_0 = 16$  shells (969 HO states) with the HO frequency of  $\hbar\omega_0 = 1.2 \times 41 \text{ MeV}/A^{1/3}$ . Values of the two essential physical constants, which determine the self-consistent solutions for the Gogny and Skyrme energy density functionals (EDFs), were the nucleon mass, amounting to  $\hbar^2/2m = 20.736676229 \text{ MeV fm}^2$ , and elementary charge squared of  $e^2 = 1.4399784086 \text{ MeV fm}$ . The two-body center-of-mass correction and exact Coulomb-exchange term were included [2].

## RESULTS FOR DOUBLY MAGIC NUCLEI

In addition to the results presented for  $^{208}\text{Pb}$  in Fig. 1 of the paper, Figs. 2–8 show analogous results for  $^{16}\text{O}$ ,  $^{40,48}\text{Ca}$ ,  $^{56,78}\text{Ni}$ , and  $^{100,132}\text{Sn}$ . Results obtained for the  $T > 0$  nuclei,  $^{48}\text{Ca}$ ,  $^{78}\text{Ni}$ , and  $^{132}\text{Sn}$ , are almost identical to those obtained for  $^{208}\text{Pb}$ . For the  $T = 0$  nuclei,  $^{16}\text{O}$ ,  $^{40}\text{Ca}$ ,  $^{56}\text{Ni}$ , and  $^{100}\text{Sn}$ , results obtained in function of the isoscalar Lagrange parameters,  $\lambda_0^\rho$ ,  $\lambda_0^{\Delta\rho}$ ,  $\lambda_0^\tau$ , or  $\lambda_0^J$  are again almost identical to those obtained for  $^{208}\text{Pb}$ . On the other hand, reaction of the  $T = 0$  systems to perturbations induced by the isovector Lagrange parameters,  $\lambda_1^\rho$ ,  $\lambda_1^{\Delta\rho}$ ,  $\lambda_1^\tau$ , or  $\lambda_1^J$ , is very weak. Only in these latter cases one can see tiny offsets between the left- and right-hand sides of Eq. (5) of the paper, but otherwise the dependencies on the isovector Lagrange parameters are almost identical too.

## RMS DEVIATIONS AND COVARIANCE MATRIX

In Table III, I show partial rms deviations between left- and right-hand sides of Eq. (5), calculated separately for each of the eight doubly magic nuclei. One can see that in all of the eight nuclei, the partial values do not differ very much from one another, which shows that the quality of adjustment of the coupling constants is similar across

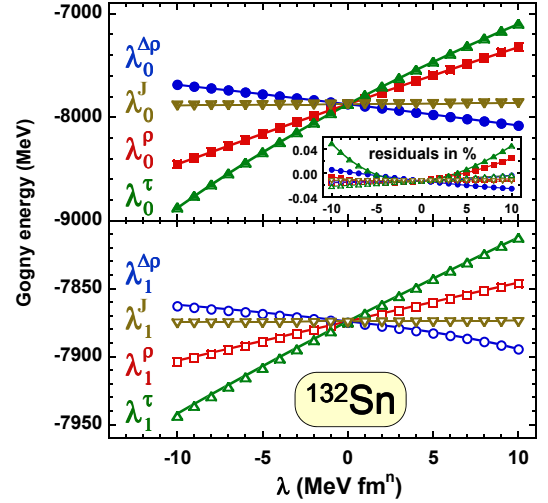

FIG. 2: (Color online) Same as in Fig. 1 of the paper, but for  $^{132}\text{Sn}$ .

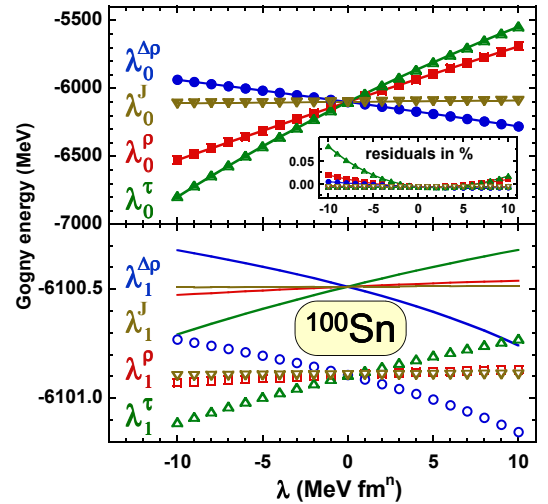

FIG. 3: (Color online) Same as in Fig. 1 of the paper, but for  $^{100}\text{Sn}$ .

the mass table. Tables IV and V show the covariance matrices [3, 4] obtained, respectively, for the eight- and six-dimensional models discussed in the paper.

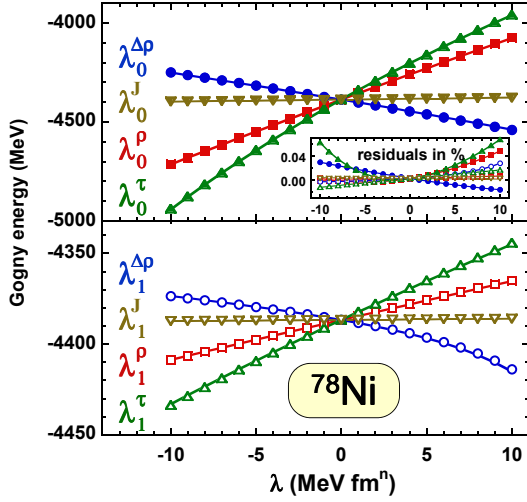

FIG. 4: (Color online) Same as in Fig. 1 of the paper, but for  $^{78}\text{Ni}$ .

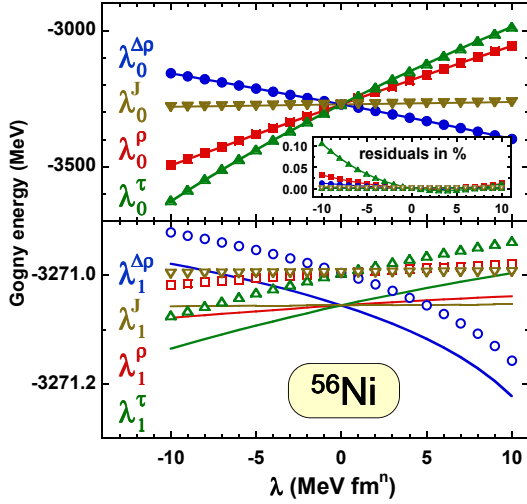

FIG. 5: (Color online) Same as in Fig. 1 of the paper, but for  $^{56}\text{Ni}$ .

## PROTON RMS RADII

In Table VI, we show the Gogny EDF D1S proton rms radii  $R_G$  compared to radii  $R$  calculated using the Skyrme EDF S1Sd, Table I of the paper.

## COMPARISON WITH THE DENSITY-MATRIX EXPANSION

Tables VII and VIII present the ground-state energies  $E$  and proton rms radii  $R$ , respectively, calculated using the original Gogny EDF D1S as compared to those obtained for the Skyrme EDF S1Sa, which was derived in Ref. [5] within the DME approximation. Tables VII and VIII are analogues of Tables II of the paper and Ta-

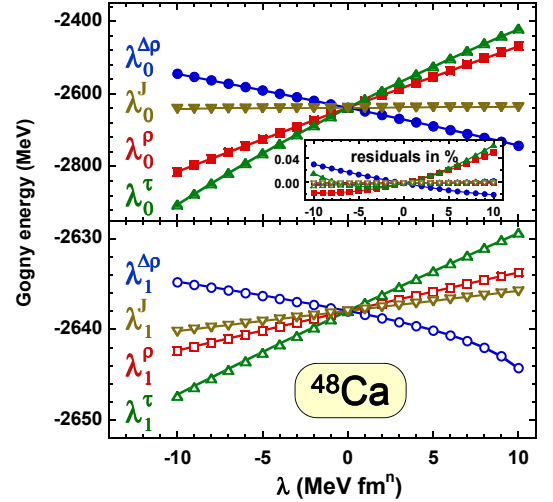

FIG. 6: (Color online) Same as in Fig. 1 of the paper, but for  $^{48}\text{Ca}$ .

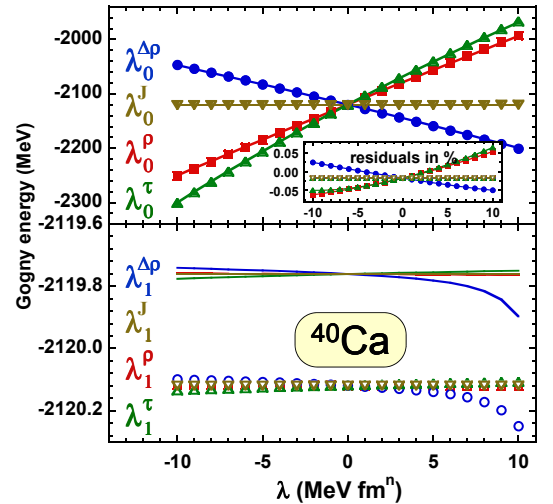

FIG. 7: (Color online) Same as in Fig. 1 of the paper, but for  $^{40}\text{Ca}$ .

ble VI, respectively.

In Ref. [5], the Gogny EDF D1S results were taken from [http://www-phynu.cea.fr/HFB-5DCH-table.htm], where no details of the numerical conditions were given. Therefore, by employing the code HFODD (v2.75c) [1], those Gogny EDF D1S results could not be exactly reproduced. In addition, in Ref. [5], the Skyrme EDF S1Sa results were obtained without taking into account the two-body center of mass correction and using the Slater approximation for the Coulomb exchange term. Therefore, the overall agreement between the Gogny EDF D1S and Skyrme EDF S1Sa results obtained there was much better than that now shown in Table VII.

One can see that the DME approximation reproduces the Gogny EDF D1S energies up to 4.83%, whereas the *ab initio*-equivalent Skyrme EDF S1Sd, presented in the

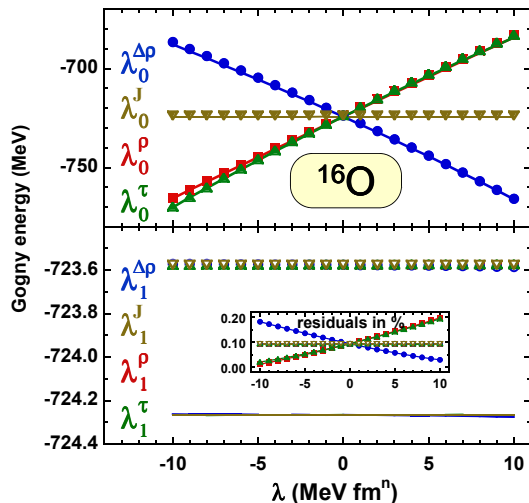

FIG. 8: (Color online) Same as in Fig. 1 of the paper, but for  $^{16}\text{O}$ .

TABLE III: Partial rms deviations between left- and right-hand sides of Eq. (4) of the paper (in MeV). Columns (b) and (c) show results obtained for the eight- and six-dimensional models, respectively.

|                   | eight-dimensional | six-dimensional |
|-------------------|-------------------|-----------------|
| (a)               | (b)               | (c)             |
| $^{16}\text{O}$   | 0.73              | 1.34            |
| $^{40}\text{Ca}$  | 0.53              | 1.15            |
| $^{48}\text{Ca}$  | 0.33              | 1.36            |
| $^{56}\text{Ni}$  | 0.52              | 0.87            |
| $^{78}\text{Ni}$  | 0.67              | 1.02            |
| $^{100}\text{Sn}$ | 0.77              | 1.15            |
| $^{132}\text{Sn}$ | 1.14              | 1.27            |
| $^{208}\text{Pb}$ | 1.45              | 1.63            |
| total             | 0.84              | 1.24            |

paper, gives the accuracy of 0.28%, that is, more than one order of magnitude better.

#### SIX-DIMENSIONAL MODEL GIVEN BY SKYRME EDF S1SE

In Tables IX and X, we repeat results given in Table II of the paper and Table VI, but for the six-dimensional model given by Skyrme EDF S1Se, see Table I of the paper.

- 
- [1] N. Schunck, J. Dobaczewski, W. Satuła, P. Bączyk, V.N. Denisov, J. Dudek, Y. Gao, M. Konieczka, T. Lesinski, K. Sato, Y. Shi, X.B. Wang, T.R. Werner, to be submitted to Computer Physics Communications.
  - [2] M. Bender, P.-H. Heenen, and P.-G. Reinhard, Rev. Mod. Phys. **75**, 121 (2003).
  - [3] J. Toivanen, J. Dobaczewski, M. Kortelainen, and K. Mizuyama, Phys. Rev. C **78**, 034306 (2008).
  - [4] J. Dobaczewski, W. Nazarewicz, and P.-G. Reinhard, J. Phys. G: Nucl. Part. Phys. **41** 074001 (2014).
  - [5] J. Dobaczewski, B.G. Carlsson, and M. Kortelainen, J. Phys. G: Nucl. Part. Phys. **37**, 075106 (2010).

TABLE IV: Covariance matrix of the eight-dimensional model leading to the Skyrme EDF S1Sd.

|                    | $C_0^\rho$    | $C_1^\rho$    | $C_0^{\Delta\rho}$ | $C_1^{\Delta\rho}$ | $C_0^\tau$    | $C_1^\tau$    | $C_0^J$       | $C_1^J$       |
|--------------------|---------------|---------------|--------------------|--------------------|---------------|---------------|---------------|---------------|
| $C_0^\rho$         | 0.477288E-01  | -0.857829E+00 | 0.264472E-01       | -0.400771E+00      | -0.496176E-01 | 0.563672E+00  | 0.179713E+00  | -0.285747E-01 |
| $C_1^\rho$         | -0.857829E+00 | 0.196409E+02  | -0.456330E+00      | 0.909189E+01       | 0.900695E+00  | -0.128445E+02 | -0.335995E+01 | 0.125789E+01  |
| $C_0^{\Delta\rho}$ | 0.264472E-01  | -0.456330E+00 | 0.206558E-01       | -0.283242E+00      | -0.256647E-01 | 0.279805E+00  | 0.105903E+00  | 0.465046E-01  |
| $C_1^{\Delta\rho}$ | -0.400771E+00 | 0.909189E+01  | -0.283242E+00      | 0.663815E+01       | 0.383224E+00  | -0.536642E+01 | -0.771368E+00 | 0.177716E+01  |
| $C_0^\tau$         | -0.496176E-01 | 0.900695E+00  | -0.256647E-01      | 0.383224E+00       | 0.524076E-01  | -0.602127E+00 | -0.198245E+00 | 0.288078E-01  |
| $C_1^\tau$         | 0.563672E+00  | -0.128445E+02 | 0.279805E+00       | -0.536642E+01      | -0.602127E+00 | 0.855370E+01  | 0.238668E+01  | -0.629264E+00 |
| $C_0^J$            | 0.179713E+00  | -0.335995E+01 | 0.105903E+00       | -0.771368E+00      | -0.198245E+00 | 0.238668E+01  | 0.145812E+01  | 0.942914E+00  |
| $C_1^J$            | -0.285747E-01 | 0.125789E+01  | 0.465046E-01       | 0.177716E+01       | 0.288078E-01  | -0.629264E+00 | 0.942914E+00  | 0.709707E+01  |

TABLE V: Covariance matrix of the six-dimensional model leading to the Skyrme EDF S1Se.

|                    | $C_0^\rho$    | $C_1^\rho$    | $C_0^{\Delta\rho}$ | $C_1^{\Delta\rho}$ | $C_0^\tau$    | $C_1^\tau$    |
|--------------------|---------------|---------------|--------------------|--------------------|---------------|---------------|
| $C_0^\rho$         | 0.253152E-01  | -0.425686E+00 | 0.142401E-01       | -0.283991E+00      | -0.246678E-01 | 0.258320E+00  |
| $C_1^\rho$         | -0.425686E+00 | 0.113067E+02  | -0.223970E+00      | 0.665050E+01       | 0.420798E+00  | -0.698582E+01 |
| $C_0^{\Delta\rho}$ | 0.142401E-01  | -0.223970E+00 | 0.150025E-01       | -0.250035E+00      | -0.115848E-01 | 0.108427E+00  |
| $C_1^{\Delta\rho}$ | -0.283991E+00 | 0.665050E+01  | -0.250035E+00      | 0.603603E+01       | 0.246589E+00  | -0.359702E+01 |
| $C_0^\tau$         | -0.246678E-01 | 0.420798E+00  | -0.115848E-01      | 0.246589E+00       | 0.248372E-01  | -0.265278E+00 |
| $C_1^\tau$         | 0.258320E+00  | -0.698582E+01 | 0.108427E+00       | -0.359702E+01      | -0.265278E+00 | 0.445782E+01  |

TABLE VI: Same as in Table II of the paper but for the proton rms radii in fm.

|                   | $R_G$  | $R$        | $\delta R$ | $\delta R/R$ | $\delta R/\Delta R$ |
|-------------------|--------|------------|------------|--------------|---------------------|
| (a)               | (b)    | (c)        | (d)        | (e)          | (f)                 |
| $^{16}\text{O}$   | 2.6689 | 2.6271(7)  | -0.0419    | -1.57%       | -64                 |
| $^{40}\text{Ca}$  | 3.4117 | 3.3763(09) | -0.0353    | -1.04%       | -41                 |
| $^{48}\text{Ca}$  | 3.4423 | 3.4261(11) | -0.0162    | -0.47%       | -15                 |
| $^{56}\text{Ni}$  | 3.6773 | 3.6732(09) | -0.0040    | -0.11%       | -4                  |
| $^{78}\text{Ni}$  | 3.9070 | 3.9104(11) | 0.0033     | 0.09%        | 3                   |
| $^{100}\text{Sn}$ | 4.4070 | 4.4033(11) | -0.0036    | -0.08%       | -3                  |
| $^{132}\text{Sn}$ | 4.6530 | 4.6568(12) | 0.0038     | 0.08%        | 3                   |
| $^{208}\text{Pb}$ | 5.4365 | 5.4394(13) | 0.0029     | 0.05%        | 2                   |
| rms               | n.a.   | n.a.       | 0.0204     | 0.69%        | 27                  |

TABLE VII: Same as in Table II of the paper but the Skyrme EDF S1Sa, which was derived in Ref. [5] within the DME approximation.

|                   | $E_G$     | $E$       | $\delta E$ | $\delta E/ E $ |
|-------------------|-----------|-----------|------------|----------------|
| (a)               | (b)       | (c)       | (d)        | (e)            |
| $^{16}\text{O}$   | -129.626  | -118.811  | 10.815     | 8.34%          |
| $^{40}\text{Ca}$  | -344.663  | -327.513  | 17.150     | 4.98%          |
| $^{48}\text{Ca}$  | -416.829  | -397.281  | 19.548     | 4.69%          |
| $^{56}\text{Ni}$  | -483.820  | -460.186  | 23.633     | 4.88%          |
| $^{78}\text{Ni}$  | -640.598  | -615.185  | 25.413     | 3.97%          |
| $^{100}\text{Sn}$ | -830.896  | -799.329  | 31.566     | 3.80%          |
| $^{132}\text{Sn}$ | -1103.246 | -1069.446 | 33.800     | 3.06%          |
| $^{208}\text{Pb}$ | -1638.330 | -1594.856 | 43.474     | 2.65%          |
| rms               | n.a.      | n.a.      | 27.446     | 4.83%          |

TABLE VIII: Same as in Table VII but for the proton rms radii in fm.

|                   | $R_G$  | $R$    | $\delta R$ | $\delta R/R$ |
|-------------------|--------|--------|------------|--------------|
| (a)               | (b)    | (c)    | (d)        | (e)          |
| $^{16}\text{O}$   | 2.6689 | 2.6822 | 0.0133     | 0.50%        |
| $^{40}\text{Ca}$  | 3.4117 | 3.4135 | 0.0018     | 0.05%        |
| $^{48}\text{Ca}$  | 3.4423 | 3.4508 | 0.0085     | 0.25%        |
| $^{56}\text{Ni}$  | 3.6773 | 3.7053 | 0.0280     | 0.76%        |
| $^{78}\text{Ni}$  | 3.9070 | 3.9231 | 0.0161     | 0.41%        |
| $^{100}\text{Sn}$ | 4.4070 | 4.4252 | 0.0182     | 0.41%        |
| $^{132}\text{Sn}$ | 4.6530 | 4.6638 | 0.0108     | 0.23%        |
| $^{208}\text{Pb}$ | 5.4365 | 5.4423 | 0.0059     | 0.11%        |
| rms               | n.a.   | n.a.   | 0.0149     | 0.40%        |

TABLE IX: Same as in Table II of the paper but the six-dimensional model given by Skyrme EDF S1Se, see Table I of the paper.

|                   | $E_G$     | $E$          | $\delta E$ | $\delta E/ E $ | $\delta E/\Delta E$ |
|-------------------|-----------|--------------|------------|----------------|---------------------|
| (a)               | (b)       | (c)          | (d)        | (e)            | (f)                 |
| $^{16}\text{O}$   | -129.626  | -128.83(6)   | 0.79       | 0.61%          | 13                  |
| $^{40}\text{Ca}$  | -344.663  | -344.34(6)   | 0.32       | 0.09%          | 5                   |
| $^{48}\text{Ca}$  | -416.829  | -419.36(7)   | -2.53      | -0.61%         | -37                 |
| $^{56}\text{Ni}$  | -483.820  | -485.83(7)   | -2.01      | -0.42%         | -29                 |
| $^{78}\text{Ni}$  | -640.598  | -642.99(13)  | -2.39      | -0.37%         | -18                 |
| $^{100}\text{Sn}$ | -830.896  | -832.60(10)  | -1.70      | -0.20%         | -18                 |
| $^{132}\text{Sn}$ | -1103.246 | -1107.17(15) | -3.93      | -0.36%         | -26                 |
| $^{208}\text{Pb}$ | -1638.330 | -1641.26(16) | -2.93      | -0.18%         | -18                 |
| rms               | n.a.      | n.a.         | 2.34       | 0.40%          | 22                  |

TABLE X: Same as in Table IX but for the proton rms radii in fm.

|                   | $R_G$  | $R$        | $\delta R$ | $\delta R/R$ | $\delta R/\Delta R$ |
|-------------------|--------|------------|------------|--------------|---------------------|
| (a)               | (b)    | (c)        | (d)        | (e)          | (f)                 |
| $^{16}\text{O}$   | 2.6689 | 2.6350(7)  | -0.0339    | -1.27%       | -48                 |
| $^{40}\text{Ca}$  | 3.4117 | 3.3860(8)  | -0.0257    | -0.75%       | -31                 |
| $^{48}\text{Ca}$  | 3.4423 | 3.4347(10) | -0.0076    | -0.22%       | -8                  |
| $^{56}\text{Ni}$  | 3.6773 | 3.6781(11) | 0.0008     | 0.02%        | 1                   |
| $^{78}\text{Ni}$  | 3.9070 | 3.9222(10) | 0.0151     | 0.39%        | 16                  |
| $^{100}\text{Sn}$ | 4.4070 | 4.4118(12) | 0.0048     | 0.11%        | 4                   |
| $^{132}\text{Sn}$ | 4.6530 | 4.6694(11) | 0.0164     | 0.35%        | 15                  |
| $^{208}\text{Pb}$ | 5.4365 | 5.4535(12) | 0.0170     | 0.31%        | 14                  |
| rms               | n.a.   | n.a.       | 0.0183     | 0.57%        | 22                  |
